# Supplementary material for: Recovery of transversely-isotropic elastic material parameters in induction motor rotors
Source: arXiv:2405.06388 source file (2024-05-10)
Supplement: Supplementary file 1 [file appendix.tex]

\section{Appendix}\label{app:stress-strain}
We now attempt to write an explicit equation to describe the compliance form of the stress-strain relation for transversely isotropic materials with compliance tensor \eqref{eq:comp_tIsotropic}. We start by writing out Hooke's law \eqref{eq:Hookes_comp} explicitly, with
\begin{equation}
\begin{aligned}
\bar{\strainInd}_1 &= \frac{1}{2G_{xy}} \bar{\stressInd}_1  - \left(\frac{1}{2G_{xy}}-\frac{1}{E_x}\right) \mathrm{tr}(\stress) - \left( \frac{1+\nu_{xz}}{E_x}-\frac{1}{2G_{xy}}\right)\bar\stressInd_3,\\
\bar{\strainInd}_2 &= \frac{1}{2G_{xy}} \bar{\stressInd}_2  - \left(\frac{1}{2G_{xy}}-\frac{1}{E_x} \right)\mathrm{tr}(\stress) - \left( \frac{1+\nu_{xz}}{E_x}-\frac{1}{2G_{xy}}\right)\bar\stressInd_3, \\
\bar{\strainInd}_3 &= \frac{E_x+E_z\nu_{xz}}{E_xE_z} \bar{\stressInd}_3  - \frac{\nu_{xz}}{E_x} \mathrm{tr}(\stress), \\
\bar{\strainInd}_4 &= \frac{1}{2G_{xz}} \bar{\stressInd}_4,\\
\bar{\strainInd}_5 &= \frac{1}{2G_{xz}} \bar{\stressInd}_5, \\
\bar{\strainInd}_6 &= \frac{1}{2G_{xy}} \bar{\stressInd}_6.
\end{aligned}
\end{equation}
% \begin{equation}
% \begin{aligned}
% \bar{\strainInd}_1 &= \frac{1}{2G_x} \bar{\stressInd}_1  - \frac{\nu_{x}}{E_x} \mathrm{tr}(\stress) - \left( \frac{\nu_{zx}}{E_z}-\frac{\nu_x}{E_x}\right)\bar\stressInd_3,\\
% \bar{\strainInd}_2 &= \frac{1}{2G_x} \bar{\stressInd}_2  - \frac{\nu_{x}}{E_x} \mathrm{tr}(\stress) - \left( \frac{\nu_{zx}}{E_z}-\frac{\nu_x}{E_x}\right)\bar\stressInd_3, \\
% \bar{\strainInd}_3 &= \frac{1}{2\mu_z} \bar{\stressInd}_3  - \frac{\nu_{zx}}{E_z} \mathrm{tr}(\stress), \\
% \bar{\strainInd}_4 &= \frac{1}{2G_x} \bar{\stressInd}_4,\\
% \bar{\strainInd}_5 &= \frac{1}{2G_{xz}} \bar{\stressInd}_5, \\
% \bar{\strainInd}_6 &= \frac{1}{2G_{xz}} \bar{\stressInd}_6,
% \end{aligned}
% \end{equation}
% where
% \begin{equation}
% \begin{aligned}
%     \mu_z &= \frac{E_z}{2(1+\nu_{zx})}.
% \end{aligned}
% \end{equation}
Decomposing $\stress$ into a block diagonal matrix 
\begin{equation}
    \stress = \begin{bmatrix}
    \stress_{11} & \stress_{12} \\ 
    \stress_{21} & \stress_{22}
    \end{bmatrix},
\end{equation}
where $\stress_{11}\in \R^{2\times 2}$, and denoting the block diagonal component
\begin{equation}
    \stress_D = \begin{bmatrix}
    \stress_{11} & \mathbf{O} \\ 
    \mathbf{O} & \stress_{22}
    \end{bmatrix},
\end{equation}
we have that 
\begin{equation} \label{eq:strain_stress_Tisotropic}
\begin{aligned} 
\strain &= \frac{1}{2}\begin{bmatrix}\frac{1}{G_{xy}} & 0 & 0 \\
0 & \frac{1}{G_{xy}} & 0 \\ 
0 & 0 & \frac{2(E_x+E_z\nu_{xz})}{E_xE_z}\end{bmatrix} \stress_D + \frac{1}{2G_{xz}}(\stress-\stress_D) - \bar{\stressInd}_3   \left( \frac{1+\nu_{xz}}{E_x}-\frac{1}{2G_{xy}}\right)   \begin{bmatrix}1 & 0 & 0 \\
0 & 1 & 0 \\ 
0 & 0 & 0 \end{bmatrix} \\
&- \begin{bmatrix}\frac{1}{2G_{xy}}-\frac{1}{E_x} & 0 & 0 \\
0 & \frac{1}{2G_{xy}}-\frac{1}{E_x} & 0 \\ 
0 & 0 & \frac{\nu_{xz}}{E_x} \end{bmatrix} \mathrm{tr}(\stress).
\end{aligned}
\end{equation}
% \begin{equation} \label{eq:strain_stress_Tisotropic}
% \begin{aligned} 
% \strain &= \frac{1}{2}\begin{bmatrix}\frac{1}{G_x} & 0 & 0 \\
% 0 & \frac{1}{G_x} & 0 \\ 
% 0 & 0 & \frac{1}{\mu_z} \end{bmatrix} \stress_D + \frac{1}{2G_{xz}}(\stress-\stress_D) - \bar{\stressInd}_3   \left( \frac{\nu_{zx}}{E_z}-\frac{\nu_x}{E_x}\right)   \begin{bmatrix}1 & 0 & 0 \\
% 0 & 1 & 0 \\ 
% 0 & 0 & 0 \end{bmatrix} \\
% &- \begin{bmatrix}\frac{\nu_x}{E_x} & 0 & 0 \\
% 0 & \frac{\nu_x}{E_x} & 0 \\ 
% 0 & 0 & \frac{\nu_{zx}}{E_z} \end{bmatrix} \mathrm{tr}(\stress).
% \end{aligned}
% \end{equation}
Alternatively, we may also express $\stress$ in terms of $\strain$. This is done by first computing 
\begin{equation}\nonumber
\mathbf{\bar{S}}^{-1} = \begin{bmatrix}
    \mathbf{\bar{S}}_1^{-1} & \mathbf{0}\\
    \mathbf{0}  & \mathbf{\bar{S}}_2^{-1}
\end{bmatrix},
\end{equation}
where, the upper and lower $3\times 3$ blocks of $\mathbf{\bar{S}}$ are given by
\begin{equation}\nonumber
\begin{aligned}
    \mathbf{\bar{S}}_1 &= \begin{bmatrix}
           \frac{1}{E_x} & \frac{1}{E_x}-\frac{1}{2G_{xy}} & -\frac{\nu_{xz}}{E_x} \\
    \frac{1}{E_x}-\frac{1}{2G_{xy}} & \frac{1}{E_x} & -\frac{\nu_{xz}}{E_x} \\
    -\frac{\nu_{xz}}{E_p} & -\frac{\nu_{xz}}{E_x} & \frac{1}{E_z}\\
    \end{bmatrix},\\
\mathbf{\bar{S}}_2 &= \begin{bmatrix}
\frac{1}{2G_{xz}} & 0 & 0 \\
0 & \frac{1}{2G_{xz}} & 0 \\
0 & 0 & \frac{1}{2G_{xy}} 
    \end{bmatrix}.
    \end{aligned}
\end{equation}
After performing some computations, we find that
\begin{equation}\nonumber
\mathbf{\bar{S}}_1^{-1} = K(\mathbf{p})
\begin{bmatrix}
 4G_x\left(\nu_{xz}^2E_z - E_x\right)& -4G_x\nu_{xz}^2E_z+4G_xE_x-2E_x^2 & -2\nu_{xz}E_xE_z \\
-4G_x\nu_{xz}^2E_z+4G_xE_x-2E_x^2 & 4G_x\left(\nu_{xz}^2E_z-E_x\right) & -2\nu_{xz}E_xE_z\\
-2\nu_{xz}E_xE_z & -2\nu_{xz}E_xE_z & \frac{E_x^2}{G_x}E_z - 4E_xE_z \\
\end{bmatrix},
\end{equation}
where 
\begin{equation}\nonumber
    K(\mathbf{p}) =  \frac{G_{xy}}{E_x^2 -4G_{xy}\left(E_x-\nu_{xz}^2E_z\right)},
\end{equation}
and
\begin{equation}\nonumber
\mathbf{\bar{S}}_2^{-1} = \begin{bmatrix}
    2G_{xz} & 0 & 0 \\
    0 & 2G_{xz} & 0 \\
    0 & 0 & 2G_{xy}
\end{bmatrix}.
\end{equation}
In this case, the explicit expression of Hooke's law is given by 
\begin{equation}
\begin{aligned}
\bar{\stressInd}_1 &= 2K(\mathbf{p}) \left(E_x^2\bar{\strainInd}_1 -(2G_x\nu_{xz}^2E_z+2G_xE_x-E_x^2)\mathrm{tr}(\strain)-(\nu_{xz}E_xE_z- 2G_x\nu_{xz}^2E_z-2G_xE_x+E_x^2)\bar{\strainInd}_3 \right),\\
\bar{\stressInd}_2 &= 2K(\mathbf{p}) \left(E_x^2\bar{\strainInd}_2-(2G_x\nu_{xz}^2E_z+2G_xE_x-E_x^2)\mathrm{tr}(\strain)-(\nu_{xz}E_xE_z- 2G_x\nu_{xz}^2E_z-2G_xE_x+E_x^2)\bar{\strainInd}_3 \right), \\
\bar{\stressInd}_3 &= 2K(\mathbf{p}) \left(\left(\frac{E_x^2}{2G_x}E_z+\nu_{xz}E_xE_z-2E_xE_z\right)\bar{\strainInd}_3-\nu_{xz}E_xE_z\mathrm{tr}(\strain)\right), \\
\bar{\stressInd}_4 &= 2G_{xz} \bar{\strainInd}_4,\\
\bar{\stressInd}_5 &= 2G_{xz} \bar{\strainInd}_5, \\
\bar{\stressInd}_6 &= 2G_{xy} \bar{\strainInd}_6,
\end{aligned}
\end{equation}

% \begin{equation}
% \mathbf{\bar{S}}^{-1} = \frac{1}{E_p^2 -4G_p\left(E_p-\nu_{pz}^2E_z\right)} 
% \begin{bmatrix}
%  4\left(G_p^2\nu_{pz}^2E_z - G_p^2E_p\right)& 2\left(-2G_p^2\nu_{pz}^2E_z+2G_p^2E_p-G_pE_p^2\right) & -2G_p\nu_{pz}E_pE_z \\
% 2\left(-2G_p^2\nu_{pz}^2E_z+2G_p^2E_p-G_pE_p^2\right) & 4\left(G_p^2\nu_{pz}^2E_z-G_p^2E_p\right) & -2G_p\nu_{pz}E_pE_z\\
% -2G_p\nu_{pz}E_pE_z & -2G_p\nu_{pz}E_pE_z & E_p^2E_z - 4G_pE_pE_z \\
% \end{bmatrix}
% \end{equation}
